# Supplementary material for: Mapping the Design Space of Teachable Social Media Feed Experiences
Source: arXiv:2401.14000 source file (2024-01-29)
Supplement: Supplementary file 1 [file appendix.tex]

\newpage
\section{Taxonomy Label Definitions}
\label{a:definitions}

\subsection{Account-Based Labels}

\begin{table*}[h]
\centering
    \begin{tabular}{p{7cm} p{7cm}}
    \toprule 
    Label & Definition\\
    \midrule 

    \multicolumn{2}{l}{\textbf{Features}} \\
    \quad The original poster & The account that published an original post. \\
    \quad The ``liker'' & The account that liked an original or reshared post. \\
    \quad The ``resharer'' & The account that reshared an original post, possibly with some added commentary. \\
    \quad The ``replier'' & The account that commented on an original or reshared post. \\

    \multicolumn{2}{l}{\textbf{Characteristics}} \\
    \quad knows personally & The participant personally knows the individual(s) running the account. \\
    \quad is a complete stranger & The participant personally has never heard of the account nor the individual(s) running it. \\
    \quad recognizes due to network effects (but does not follow) & The participant has heard of or previously encountered the account via their network but does not follow it. \\
    \quad following out of specific topical interest & The participant follows the account for a specific topic they are interested in. \\
    \quad following out of general interest & The participant follows the account because they are generally interested in the account's content without articulating a specific topic. \\
    \quad following due to past enjoyable content & The participant follows the account because they enjoyed content the platform previously posted, independent of whether it aligns with their interests. \\
    \quad following due to admirable/significant personal trait & The participant follows the account because they find significance and/or admiration in a personal trait of individual(s) running the account. \\
    \quad has shifted away from being relevant & The account was initially of interest to the participant but became less so over time. \\
    \quad posts infrequently & The participant perceives the account to be posting infrequently. \\
    \quad posts frequently & The participant perceives the account to be posting frequently. \\
    
    \bottomrule
    \end{tabular}
    \caption{Our definitions for labels in our account-based taxonomies.}
    \label{t:acct-label-defs}
    \Description{A 2-column table with headings Label and Definition. Labels are categorized into features and characteristics. There are 4 features and 10 characteristics. Each label has its own definition in the same row.}
\end{table*}

\subsection{Content-Based Labels}

\begin{table*}[h]
\centering
    \begin{tabular}{p{5cm} p{9cm}}
    \toprule 
    Label & Definition\\
    \midrule 

    \multicolumn{2}{l}{\textbf{Features}} \\
    \quad Content (all-inclusive/unspecified) & General reference to the content without further specification of its features. \\
    \quad Body text content & The text in the main body of the post (i.e. not embedded into an image or video). \\
    \quad Image content & Image(s) attached to a post. \\
    \quad Video content & Video(s) attached to a post. \\
    \quad Multimodal content & Media within a post that have a combination of two or more of the following: text, image, video, audio. Unlike image or video, his label is only applied if a participant specifically mentions using multimodality as a signal. \\
    \quad Topic & Topic(s) that participants interpret or directly obtain from a post. \\
    \quad Accounts mentioned & Account(s) that are mentioned in the post body. Note that this is a content-based feature distinct from accounts that post/reshare/like/reply to posts. \\
    \quad Link(s) & Clickable hyperlinks included in the post. \\
    \quad Hashtag(s) & Text-based hashtags included in a post. \\

    \multicolumn{2}{l}{\textbf{Characteristics}} \\
    \quad contains an existing personal interest & The content contains an existing interest that arose from a participant's personal life. \\
    \quad contains an existing professional interest & The content contains an existing interest that arose from a participant's professional life. \\
    \quad contains a potential interest (personal or professional) & The content piques a participant's interest, but is not yet aligned with an existing interest. \\
    \quad contains a topic/opinion I want to avoid & The participant identifies topics or opinions within the post they would rather not consume. \\
    \quad is irrelevant to me & The content is considered irrelevant by the participant.  \\
    \quad is time-sensitive and relevant & The participant identifies a time-sensitive aspect of the post that makes it relevant. \\
    \quad related to ads and consumerism & The content is perceived to contain ads and/or is prompting purchases. \\
    \quad belongs to a notable trend/genre & The content is created in accordance with a notable trend and/or genre identified by the participant. \\
    \quad geographically relevant & The content is relevant because it discusses subjects geographically local to the participant. \\
    \quad is funny & The participant considers the content funny. \\
    \quad is relatable & The participant considers the content relatable. \\
    \quad invokes positive emotions & The participant reports feeling positive emotions after consuming the content. \\
    \quad invokes negative emotions & The participant reports feeling negative emotions after consuming the content. \\
    \quad is informative and/or educational & The participant considers the content to be informative or have educational value. \\
    \quad lacks information or context & The participant desires more information or context from the content. \\
    \quad is of low quality and/or repetitive & The participant considers the content to be low quality and/or too similar with previously seen content. \\
    \quad high (long, cognitively demanding) & The participant felt that consuming the content was rather effortful. \\
    \quad low (short, straightforward) & The participant felt that consuming the content was rather effortless. \\
    
    \bottomrule
    \end{tabular}
    \caption{Our definitions for labels in our content-based taxonomies.}
    \label{t:content-label-defs}
    \Description{A 2-column table with headings Label and Definition. Labels are categorized into features and characteristics. There are 4 features and 10 characteristics. Each label has its own definition in the same row.}
\end{table*}

\section{Disaggregated Taxonomies}
\label{a:disaggregated}

\subsection{Disaggregated Account-Based Taxonomies}
\begin{figure}[h]
    \centering
    \includegraphics[width=1\textwidth]{Taxonomy distilled - InstagramAccount.pdf}
    \caption{Account-based taxonomy for Instagram. Note that Instagram does not include in-feed affordances to view content ``resharers,'' which we indicate with the patterned row.}
\end{figure}

\begin{figure}[h]
    \centering
    \includegraphics[width=1\textwidth]{Taxonomy distilled - MastodonAccount.pdf}
    \caption{Account-based taxonomy for Mastodon.}
\end{figure}

\begin{figure}[h]
    \centering
    \includegraphics[width=1\textwidth]{Taxonomy distilled - TikTokAccount.pdf}
    \caption{Account-based taxonomy for TikTok. Note that TikTok does not include in-feed affordances to view content ``likers'' and ``resharers,'' which we indicate with the patterned rows.}
\end{figure}

\begin{figure}[h]
    \centering
    \includegraphics[width=1\textwidth]{Taxonomy distilled - TwitterAccount.pdf}
    \caption{Account-based taxonomy for Twitter.}
\end{figure}

\subsection{Disaggregated Content-Based Taxonomies}
\begin{figure}[h]
    \centering
    \includegraphics[width=1\textwidth]{Taxonomy distilled - InstagramContent.pdf}
    \caption{Content-based taxonomy for Instagram.}
\end{figure}

\begin{figure}[h]
    \centering
    \includegraphics[width=1\textwidth]{Taxonomy distilled - MastodonContent.pdf}
    \caption{Content-based taxonomy for Mastodon.}
\end{figure}

\begin{figure}[h]
    \centering
    \includegraphics[width=1\textwidth]{Taxonomy distilled - TikTokContent.pdf}
    \caption{Content-based taxonomy for TikTok.}
\end{figure}

\begin{figure}[h]
    \centering
    \includegraphics[width=1\textwidth]{Taxonomy distilled - TwitterContent.pdf}
    \caption{Content-based taxonomy for Twitter.}
\end{figure}
